# Supplementary material for: Empowering the Quantum Cloud User with QRIO
Source: arXiv:2407.17676 source file (2024-07-26)
Supplement: Supplementary file 1 [file Appendix.tex]

\section{Artifact Appendix}

%%%%%%%%%%%%%%%%%%%%%%%%%%%%%%%%%%%%%%%%%%%%%%%%%%%%%%%%%%%%%%%%%%%%%
\subsection{Abstract}

{\em Quantum computing is moving swiftly from theoretical to practical applications, making it crucial to establish a significant quantum advantage. Despite substantial investments, access to quantum devices is still limited, with users facing issues like long wait times and inefficient resource management. Unlike the mature cloud solutions for classical computing, quantum computing lacks effective infrastructure for resource optimization. 

We propose a Quantum Resource Infrastructure Orchestrator (QRIO), a state-of-the-art cloud resource manager built on Kubernetes that is tailored to quantum computing. QRIO seeks to democratize access to quantum devices by providing customizable, user-friendly, open-source resource management. QRIO's design aims to ensure equitable access, optimize resource utilization, and support diverse applications, thereby speeding up innovation and making quantum computing more accessible and efficient to a broader user base. In this paper, we discuss QRIO's various features and evaluate its capability on several representative usecases. QRIO's code and demo video can be found at \textcolor{blue}{{https://anonymous.4open.science/r/QRIO-Components-595E/}}.}

\subsection{Artifact check-list (meta-information)}

{\small
\begin{itemize}
  \item {\bf Hardware: Apple Macbook with 18 GB RAM and at least 120 GB free space in }
  \item {\bf Experiments: 5 }
  \item {\bf How much disk space required (approximately)?: at least 150 GB }
  \item {\bf How much time is needed to prepare workflow (approximately)?: 1 - 1.5 hrs}
  \item {\bf How much time is needed to complete experiments (approximately)?: 1 - 2 hrs }
  \item {\bf Publicly available?: Yes }
  \item {\bf Workflow framework used?: React JS, Node JS, Django, Docker, Kubernetes, Minikube}
\end{itemize}
}

%%%%%%%%%%%%%%%%%%%%%%%%%%%%%%%%%%%%%%%%%%%%%%%%%%%%%%%%%%%%%%%%%%%%%

\subsubsection{How to access}
The artifact can be access on this url: \textcolor{blue}{{https://anonymous.4open.science/r/QRIO-Components-595E/}}

\subsubsection{Hardware dependencies}
We recommend running the software on at least 16-18 GB of RAM and having at least 120 GB of storage available for smooth results. Moreover, we tested the system of an Apple MacBook Pro with M3 Pro chip 18 GB RAM and 512 GB memory.

\subsubsection{Software dependencies}
The software dependencies we require the evaluator to install are:
\begin{itemize}
    \item Docker
    \item Kubernetes
    \item Minikube
    \item React
    \item All dependencies mentioned in requirements.txt of QRIOMeta-Main
    \item All dependencies mentioned in package.json of QRIOVisualiser-main/backend
    \item All dependencies mentioned in package.json of QRIOVisualiser-main/frontend
\end{itemize}
% \subsubsection{Data sets}

% \subsubsection{Models}

%%%%%%%%%%%%%%%%%%%%%%%%%%%%%%%%%%%%%%%%%%%%%%%%%%%%%%%%%%%%%%%%%%%%%
\subsection{Installation}
The steps for installing the software and it dependencies have been mentioned in the Readme section of \textcolor{blue}{{https://anonymous.4open.science/r/QRIO-Components-595E/}} . The Figshare DOI is: \textcolor{blue}{10.6084/m9.figshare.26360725}

%%%%%%%%%%%%%%%%%%%%%%%%%%%%%%%%%%%%%%%%%%%%%%%%%%%%%%%%%%%%%%%%%%%%%
% \subsection{Experiment workflow}

%%%%%%%%%%%%%%%%%%%%%%%%%%%%%%%%%%%%%%%%%%%%%%%%%%%%%%%%%%%%%%%%%%%%%
\subsection{Evaluation and expected results}
The artifact should be evaluated using the following experiments and should expect the following results:

1. \textbf{Experiment 1}- This experiment is made with the goal of testing the functionality of the tool in its entirety i.e. the visualizer, the master server, meta server and the kubernetes server. When uploading bv.qasm and scheduling the file with either topology or fidelity, the output is close to the following:

\#\#\#\#\#\#\#\#\#\# Noisy Simulation \#\#\#\#\#\#\#\#\#\#
{'0000010000': 2, '0001000101': 1, '1101010001': 1, '1101010100': 1, '0101010110': 1, '0000000100': 12, '0100000101': 4, '1001000000': 1, '0001010101': 13, '0101010101': 413, '0101000100': 1, '0000000101': 9, '0001011000': 1, '0001010000': 2, '0100000000': 9, '0100010101': 6, '0101010100': 15, '0001010100': 1, '0000000000': 445, '0111010001': 1, '0111010101': 1, '0000000001': 15, '0001010001': 1, '0000010101': 1, '0101000101': 7, '0001000000': 5, '0101010000': 4, '0010000000': 6, '1101010101': 2, '0101011000': 1, '0101010001': 26, '0000100000': 4, '0000001000': 1, '1000000000': 9, '0101011101': 2}
\#\#\#\#\#\#\#\#\#\#

Also running the following command in the terminal gives the final score for each node:
Nodes final score: [List of final scores] and Kubernetes chooses the node with the highest score: this can viewed by running the command "kubectl events" and observing the scheduled tag.

2. \textbf{Experiment 2} is created with the aim of reproducing Experiment 4.4 in this paper. It will exactly reproduce the answer.

3. \textbf{Experiment 3} (is created with the aim of reproducing experiment 4.5 in the paper): This experiment shows the performance of the filtering algorithm of the scheduler on 100 quantum devices with different average two qubit error rates. This mimics the situation where the user asks for devices with a specific maximum two qubit error rate and the scheduler filters from the available devices the set of devices which satisfy the request. This experiment is to show this phenomena. The error rates of these devices are stored in the file `scheduler\_filter.py` in this folder. In the real scheduler code this is stored in a similar data structure. Since, we cannot locally run a 100 node kubernetes cluster, we went for a simulated code which perfectly simulates the filtering algorithm of the scheduler.

\textbf{Output}: \\
\[9, 18, 23, 31, 39, 44, 50, 60, 69, 77, 100 \]

The output is similar to the trends shown in experiment 4.5 in the paper. The reason for not being exactly similar is that the backends used during the original evaluation was slightly different to the ones used for the experiments documentation. The reason for this different in the non determinism in probabilistically generating the devices topologies and error rates.

4. \textbf{Experiment 4} (is created with the aim of reproducing experiment 4.2 in the paper) This experiment shows the performance of the ranking strategy of the scheduler. This basically shows that the device chosen by the scheduler has a lower score than the device chosen a random choice scheduling strategy. Semantically a lower score would mean that the device chosen by the scheduler confirms better to the device chosen randomly. Since, the scheduler always outperforms the random scheduling strategy, this experiment showcases the average decrease in score of QRIO's scheduler vs Random scheduler. This experiment is supposed to mimic the experiment 4.2 in the paper. However, there will not be an exact simulation as the devices used for the evaluation in the paper is slightly different from the devices used for this experiment. The reason for that being the non determinism in the custom backend generation algorithm. The custom backend generation algorithm uses probability to generate the error rates and topologies.

Having said that, the trend is similar in the sense that the scheduler always outperforms a random scheduling strategy.

\textbf{Output(Similar to)}: \\
full Round 0 \\
random score 0.9999858466127605 \\
lowest\_Score 0.19418617712031871 \\
\#\#\#\#\#\#\#\#\#\#\#\#\#\#\#\# \\
full Round 1 \\
random score 0.9999664725245402 \\
lowest\_Score 0.20385764418426555 \\
\#\#\#\#\#\#\#\#\#\#\#\#\#\#\#\# \\
grid Round 0 \\
random score 0.8173709749983582 \\
lowest\_Score 0.046861651948303384 \\
\#\#\#\#\#\#\#\#\#\#\#\#\#\#\#\# \\
grid Round 1 \\
random score 0.5889804427833296 \\
lowest\_Score 0.046861651948303384 \\
\#\#\#\#\#\#\#\#\#\#\#\#\#\#\#\# \\
h\_square Round 0 \\
random score 0.3849874598722839 \\
lowest\_Score 0.06946242495991461 \\
\#\#\#\#\#\#\#\#\#\#\#\#\#\#\#\# \\ 
h\_square Round 1 \\
random score 0.9999831415904125 \\
lowest\_Score 0.06946242495991461 \\
\#\#\#\#\#\#\#\#\#\#\#\#\#\#\#\# \\
line Round 0 \\
random score 0.9988985309728632 \\
lowest\_Score 0.05822983320040409 \\
\#\#\#\#\#\#\#\#\#\#\#\#\#\#\#\# \\
line Round 1 \\
random score 0.9999961464992105 \\ 
lowest\_Score 0.05822983320040409 \\
\#\#\#\#\#\#\#\#\#\#\#\#\#\#\#\# \\
ring Round 0 \\
random score 0.9948626402510966 \\
lowest\_Score 0.08056104441696343 \\ 
\#\#\#\#\#\#\#\#\#\#\#\#\#\#\#\# \\
ring Round 1 \\
random score 0.9999999999692435 \\
lowest\_Score 0.08056104441696343 \\
\#\#\#\#\#\#\#\#\#\#\#\#\#\#\#\# \\
{'full': 0.8009542489163581, 'grid': 0.6563140569425405, 'h\_square': 0.6230228757714336, 'line': 0.9412175055356328, 'ring': 0.9168702756932066} \\

As the dictionary output (which shows the average difference between the score obtained by the scheduler and the score obtained by the random scheduler) you would find the scores found by the random scheduling strategy and the QRIO scheduling strategy and also a dictionary saying the average decrease in scores of QRIO's scheduled device and the device chosen at random.

5. \textbf{Experiment 5} (is created with the aim of reproducing experiment 4.3 in the paper) from the paper should be reproducible.

This experiment evaluates the performance of QRIO for the fidelity ranking aspect of the scheduler. This basically compares the following algorithms: Random scheduler, QRIO simulated scheduler and Oracle algorithm.

Throughout the experiment we demand a 100\% fidelity. Since no device is capable of providing the fidelity requested, we give the best possible backend closes to the requested fidelity. The script gets two different fidelities the fidelity of the original circuit and the fidelity of the clifford converted circuit. The device with the best (highest) fidelity of the clifford converted circuit is the device the scheduler runs on. The device with the highest oracle fidelity is the device where the Oracle algorithm will schedule the circuit. Now, this experiment is all about proving that the original fidelity of the device where the simulated scheduler scheduled the circuit is not greater than the oracle fidelity i.e. the original fidelity of the device where the Oracle algorithm would choose to schedule the circuit. This experiment is designed to mimic the trend in experiment 4.3 in the paper. However, there will not be an exact simulation as the devices used for the evaluation in the paper is slightly different from the devices used for this experiment. The reason for that being the non determinism in the custom backend generation algorithm. The custom backend generation algorithm uses probability to generate the error rates and topologies.

Having said that, the thing to evaluate is that the trend is similar i.e. the Oracle has the best fidelity, then the fidelity of the device chosen by the scheduler, and lastly the random choice.

We also show the diagrams of converted(to clifford) and unconverted(to clifford) circuits of two qasm files bv and circ1. The thing to note here is that circ1 has some non clifford gates which are transformed after conversion to clifford. However, bv does not have such gates, so the converted and unconverted gates are similar.

\textbf{Output (Should be similar to)}:
bv Round 0 \\
random fidelity 0.0032317452299887137 \\
scheduled device fidelity 0.3820572189362527 \\
Oracle fidelity 0.3820572189362527 \\
Oracle backend backend\_87 \\
Original backend backend\_87 \\
Average fidelity 0.026677790722921556 \\
Median Fidelity 0.0032131414592208598 \\
\#\#\#\#\#\#\#\#\#\#\#\#\#\#\#\# \\
hsp Round 0 \\
random fidelity 0.35334201971849455 \\
scheduled device fidelity 0.8192678008393258 \\
Oracle fidelity 0.8192678008393258 \\
Oracle backend backend\_87 \\
Original backend backend\_87 \\
Average fidelity 0.38474741970694176 \\
Median Fidelity 0.3528701090451422 \\
\#\#\#\#\#\#\#\#\#\#\#\#\#\#\#\# \\
rep Round 0 \\
random fidelity 0.9819414098337695 \\
scheduled device fidelity 0.984077273674334 \\
Oracle fidelity 0.9903994292909956 \\
Oracle backend backend\_42 \\
Original backend backend\_1 \\
Average fidelity 0.9822250625091944 \\
Median Fidelity 0.9828074287832163 \\
\#\#\#\#\#\#\#\#\#\#\#\#\#\#\#\# \\
grover Round 0 \\
random fidelity 0.0900000000000001 \\
scheduled device fidelity 0.7488888888888888 \\
Oracle fidelity 0.7488888888888888 \\
Oracle backend backend\_42 \\
Original backend backend\_42 \\
Average fidelity 0.2132 \\
Median Fidelity 0.1305555555555556 \\
\#\#\#\#\#\#\#\#\#\#\#\#\#\#\#\# \\
circ1 Round 0 \\
random fidelity 0.8203115431384835 \\
scheduled device fidelity 0.9173805613161197 \\
Oracle fidelity 0.9173805613161197 \\
Oracle backend backend\_42 \\
Original backend backend\_42 \\
Average fidelity 0.7838041475948553 \\
Median Fidelity 0.7751766518876981 \\
\#\#\#\#\#\#\#\#\#\#\#\#\#\#\#\# \\
circ2 Round 0 \\
random fidelity 0.004444444444444502 \\
scheduled device fidelity 0.4622222222222222 \\
Oracle fidelity 0.4622222222222222 \\
Oracle backend backend\_42 \\
Original backend backend\_42 \\
Average fidelity 0.03830000000000009 \\
Median Fidelity 0.005555555555555636 \\
\#\#\#\#\#\#\#\#\#\#\#\#\#\#\#\# \\
Look at the terminal running QRIOMeta-Server and observe the logs. \\

The instructions for running the code and the experiments are available in the README attached to the submission (in the main folder and the individual Experiment folders). The main aim is that the results are reasonably reproducible. There always exists some non determinism in the process.

% {\em Obligatory}

%%%%%%%%%%%%%%%%%%%%%%%%%%%%%%%%%%%%%%%%%%%%%%%%%%%%%%%%%%%%%%%%%%%%%
% \subsection{Experiment customization}

% %%%%%%%%%%%%%%%%%%%%%%%%%%%%%%%%%%%%%%%%%%%%%%%%%%%%%%%%%%%%%%%%%%%%%
% \subsection{Notes}

%%%%%%%%%%%%%%%%%%%%%%%%%%%%%%%%%%%%%%%%%%%%%%%%%%%%%%%%%%%%%%%%%%%%%
% \subsection{Methodology}

% Submission, reviewing and badging methodology:

% % \begin{itemize}
% %   % \item \url{https://www.acm.org/publications/policies/artifact-review-badging}
% %   % \item \url{http://cTuning.org/ae/submission-20201122.html}
% %   % \item \url{http://cTuning.org/ae/reviewing-20201122.html}
% % \end{itemize}
